# Supplementary material for: Faster Sampling via Stochastic Gradient Proximal Sampler
Source: arXiv:2405.16734 source file (2024-05-27)
Supplement: Supplementary file 1 [file 04Lem_Convanybatch.tex]

\section{Investigation of Convergence for Any Batch-size.}
Inheriting notations presented in Section~\ref{sec:not_ass_0x}, we modify the update of $\{\rvx_k\}$.
In the following, we only consider one update of $\rvx_k$ where $\rvx_k$ and $\rvx_{k+1/2}$ are abbreviate as $\rvx_0$ and $\rvx_\eta$ for simplification. 

According to Eq~\ref{def:transition_kernel_stage1}, the transition kernel from $\rvx_0$ to $\rvx_\eta$, the corresponding SDE can be formulated as
\begin{equation*}
    \der \rvx_t = \der B_t,
\end{equation*}
which will be extended to  
\begin{equation}
    \label{sde:modified_sps_stage1}
    \der \rvx_t = g(t)\der B_t,
\end{equation}
in the following analysis.

According to the main idea of proximal samplers, we need to use the following analysis to obtain the transition from $\rvx_{k+1/2}$ to $\rvx_{k+1}$ abbreviated as $\rbkwx_0$ and $\rbkwx_\eta$.
First, we consider another Markov process $\{\rvz_t\}_{t\in[0,\eta]}$ with the same SDE as Eq~\ref{sde:modified_sps_stage1}, while $\rvz_0\sim p_*$.
The closed form of $\rvz_t$ can be obtained as
\begin{equation*}
    \rvz_t = \rvz_0 + \int_0^t \der \rvz_s = \rvz_0 + \int_0^t g(s)\der B_s = \rvz_0 + \xi_t\quad \mathrm{where}\quad \xi_t \sim \mathcal{N}\left(\vzero, \sigma_t^2 \cdot \mI\right).
\end{equation*}
where the variance satisfies
\begin{equation*}
    \sigma_t^2 = \int_0^t g^2(s)\der s
\end{equation*}
due to the Ito's isometry.
Therefore, the underlying distribution of $\rvz_t$ will be $q_t = p_*\ast \varphi_{\sigma_t^2}$.
Specifically, we have
\begin{equation}
    \label{ineq:q_t_density}
    q_\eta(\vz) = \int C_*^{-1}\cdot \exp(-f(\vz_0))\cdot C(\sigma_\eta^2)^{-1}\cdot \exp\left(-\frac{\left\|\vz-\vz_0\right\|^2}{2\sigma_\eta^2}\right)\der \vz_0.
\end{equation}

We suppose another Markov process $\{\bkw{\rvz}_t\}_{t\in[0,\eta]}$ satisfying $\bkw{\rvz}_t = \rvz_{\eta - t}$, we will obtain the transition kernel from $\bkw{\rvz}_0$ to $\bkw{\rvz}_\eta$ will be 
\begin{equation*}
    \bkw{q}_{\eta|0}(\vz|\vz_0) = C^{-1}(\sigma_\eta^2, \vz_0)\cdot \exp\left(-f(\vz) - \frac{\left\|\vz-\vz_0\right\|^2}{2\sigma_\eta^2}\right).
\end{equation*}
We can validate this result by checking the establishment of the following equation.
\begin{equation*}
    \scriptstyle
    \begin{aligned}
        &\int \bkw{q}_0(\vz_0) \cdot \bkw{q}_{\eta|0}(\vz|\vz_0)\der \vz_0 = \int q_\eta(\vz_0)\cdot \bkw{q}_{\eta|0}(\vz|\vz_0)\der \vz_0\\
        & =  \int \left(\int C_*^{-1}\cdot \exp(-f(\vz^\prime))\cdot C(\sigma^2_{\eta})^{-1}\cdot \exp\left(-\frac{\left\|\vz_0-\vz^\prime\right\|}{2\sigma_\eta^2}\right)\der \vz^\prime\right) \cdot C^{-1}(\sigma_\eta^2, \vz_0)\cdot \exp\left(-f(\vz) - \frac{\left\|\vz-\vz_0\right\|^2}{2\sigma_\eta^2}\right) \der \vz_0\\
        & = C_*^{-1} \cdot \exp(-f(\vz))\cdot \int \left(\underbrace{\int C^{-1}(\sigma_\eta^2,\vz_0)\cdot \exp\left(-f(\vz^\prime) - \frac{\left\|\vz_0-\vz^\prime\right\|^2}{2\sigma_\eta^2}\right)\der \vz^\prime}_{=1}\right) \cdot C(\sigma_\eta^2)^{-1} \cdot \exp\left(-\frac{\left\|\vz-\vz_0\right\|^2}{2\sigma_\eta^2}\right)\der \vz_0\\
        & = C_*^{-1}\cdot \exp(-f(\vz)) = \bkw{q}_\eta (\vz).
    \end{aligned}
\end{equation*}

Since we require the sampling subproblem to be randomized, we suppose the transition kernel from $\bkw{\rvx}_0$ to $\bkw{\rvx}_\eta$ to be 
\begin{equation*}
    \bkw{p}_{\eta|0}(\vx|\vx_0) = C^{-1}(\sigma_\eta^2, \vx_0)\cdot \exp\left(-f_{\vb}(\vx) - \frac{\left\|\vx-\vx_0\right\|^2}{2\sigma_\eta^2}\right).
\end{equation*}

With all the above prior, we start to analyze the contraction of stochastic proximal samplers following from~\cite{chen2022improved}

\paragraph{First stage analysis.}
For the first stage, we set $\phi(x) = x\log x$, which satisfies $\phi^\prime(x) = \log x + 1$. 
Since the KL divergence between $p$ and $q$ can be presented as $\KL{p}{q}= \E_q[\phi(p/q)]$, we have
\begin{equation}
    \label{ineq:kl_contraction_start}
    \begin{aligned}
        2\partial_t \KL{p_t}{q_t} = & 2 \int \left(\log \frac{p_t(\vx)}{q_t(\vx)} + 1\right)\cdot \left(\partial_t p_t(\vx) - \frac{p_t(\vx)}{q_t(\vx)}\cdot \partial_t q_t(\vx)\right) \der \vx\\
        & + 2\int \left(\frac{p_t(\vx)}{q_t(\vx)}\log \frac{p_t(\vx)}{q_t(\vx)}\right)\cdot \partial_t q_t(\vx)\der\vx.
    \end{aligned}
\end{equation}
Combining Fokker-Planck equation, Eq~\ref{sde:modified_sps_stage1}, we have
\begin{equation*}
    \begin{aligned}
        \partial_t p_t(\vx) = \Delta \left[\frac{g^2(t)}{2}p_t (\vx)\right] = \frac{g^2(t)}{2}\Delta p_t(\vx) = \frac{g^2(t)}{2}\cdot \nabla \cdot \left(p_t(\vx)\grad\log p_t(\vx)\right),\\
        \partial_t q_t(\vx) = \Delta \left[\frac{g^2(t)}{2}q_t (\vx)\right] = \frac{g^2(t)}{2}\Delta q_t(\vx)= \frac{g^2(t)}{2}\cdot \nabla \cdot \left(q_t(\vx)\grad\log q_t(\vx)\right),
    \end{aligned}
\end{equation*}
where $\nabla$ and $\Delta$ are the divergences and the Laplace operator perspectively.
Plugging this equation into Eq~\ref{ineq:kl_contraction_start}, we have
\begin{equation*}
    \begin{aligned}
        2\partial_t \KL{p_t}{q_t} & = g^2(t)\int \left(\log \frac{p_t(\vx)}{q_t(\vx)} + 1\right)\cdot \left(\nabla \cdot \left(p_t(\vx)\grad\log p_t(\vx)\right) - \frac{p_t(\vx)}{q_t(\vx)}\cdot \nabla \cdot \left(q_t(\vx)\grad\log q_t(\vx)\right)\right)\der\vx\\
        &\quad + g^2(t)\int \left(\frac{p_t(\vx)}{q_t(\vx)}\log \frac{p_t(\vx)}{q_t(\vx)}\right)\cdot \nabla \cdot \left(q_t(\vx)\grad\log q_t(\vx)\right)\der\vx\\
        &= -g^2(t)\int p_t(\vx) \left<\grad \left(\log \frac{p_t(\vx)}{q_t(\vx)} + 1\right), \grad \log p_t(\vx)\right>\der \vx\\
        &\quad + g^2(t)\int q_t(\vx)\left<\grad \left(\left(\log \frac{p_t(\vx)}{q_t(\vx)}+1\right)\cdot \frac{p_t(\vx)}{q_t(\vx)}\right), \grad \log q_t(\vx)\right> \der \vx\\
        &\quad - g^2(t)\int q_t(\vx)\left<\grad \left(\frac{p_t(\vx)}{q_t(\vx)}\log \frac{p_t(\vx)}{q_t(\vx)}\right),\grad \log q_t(\vx)\right> \der \vx\\
        &=-g^2(t)\int p_t(\vx) \left<\grad \left(\log \frac{p_t(\vx)}{q_t(\vx)} + 1\right), \grad \log \frac{p_t(\vx)}{q_t(\vx)}\right>\der \vx =-g^2(t)\FI{p_t}{q_t}.
    \end{aligned}
\end{equation*}
Besides, we should note that $q_t = p_* \ast \varphi_{\sigma^2_t}$ satisfies LSI with a constant
\begin{equation*}
    \alpha_t = \left(\frac{1}{\alpha_*}+ \frac{1}{\sigma_t^2}\right)^{-1},
\end{equation*}
which implies
\begin{equation*}
    2\partial_t \KL{p_t}{q_t}\le - \frac{\alpha_t g^2(t)}{2}\KL{p_t}{q_t} \quad \Leftrightarrow \quad \KL{p_t}{q_t} = \exp\left(-A_t\right)\KL{p_0}{q_0}.
\end{equation*}
Noted that 
\begin{equation*}
    \begin{aligned}
        A_t  =\frac{1}{2} \cdot \int_0^t \alpha_sg^2(s)\der s.
    \end{aligned}
\end{equation*}
If we choose proper $g(t)$, the forward process will decay exponentially.
However, the choice of $g(t)$ will also be dependent on the contraction of the second stage update.

\paragraph{Second stage analysis}
Then, we should investigate the second stage, which is more important.
Similar to~\cite{chen2022sampling}, we consider an interpolating SDE of $\bkw{\rvz}_t$ as
\begin{equation*}
    \der \bkw{\rvz}_t = \bkw{\vb}_t(\bkw{\rvz}_t)\der t + g(\eta - t)\der B_t
\end{equation*}
where the drift term satisfies
\begin{equation*}
    \bkw{\vb}_{\eta - t} + \vzero = g^2(t)\grad \log q_t\quad \Leftrightarrow\quad \bkw{\vb}_{t}= g^2(\eta-t)\grad\log q_{\eta - t}.
\end{equation*}
Hence, we have
\begin{equation*}
    \der \bkw{\rvz}_t = g^2(\eta - t) \grad\log q_{\eta-t}(\bkw{\rvz}_t)\der t + g(\eta - t)\der B_t.
\end{equation*}
According to the closed form of $q_t$ has presented in Eq~\ref{ineq:q_t_density}, we have
\begin{equation}
    \label{ineq:score_formula}
    \begin{aligned}
        \grad \log q_{\eta - t}(\vz) & = \frac{\grad q_{\eta-t}(\vz)}{q_{\eta-t}(\vz)} = \frac{\int C_*^{-1}\cdot \exp(-f(\vz_0))\cdot C(\sigma_{\eta-t}^2)^{-1}\cdot \exp\left(-\frac{\left\|\vz-\vz_0\right\|^2}{2\sigma_{\eta-t}^2}\right)\cdot \left(- \frac{\vz-\vz_0}{\sigma_{\eta-t}^2}\right) \der \vz_0}{\int C_*^{-1}\cdot \exp(-f(\vz_0))\cdot C(\sigma_{\eta-t}^2)^{-1}\cdot \exp\left(-\frac{\left\|\vz-\vz_0\right\|^2}{2\sigma_{\eta-t}^2}\right)\der \vz_0}\\
        & = \E_{\rvz_0\sim r_{\eta-t}(\cdot|\vz)}\left[-\frac{\vz - \rvz_0}{\sigma_{\eta-t}^2}\right].
    \end{aligned}
\end{equation}
Then, we suppose 
\begin{equation*}
    \begin{aligned}
        \grad \log q_{\eta - t|\vb}(\vx) & \coloneqq \frac{\int C_*^{-1}\cdot \exp(-f_{\vb}(\vx_0))\cdot C(\sigma_{\eta-t}^2)^{-1}\cdot \exp\left(-\frac{\left\|\vx-\vx_0\right\|^2}{2\sigma_{\eta-t}^2}\right)\cdot \left(- \frac{\vx-\vx_0}{\sigma_{\eta-t}^2}\right) \der \vx_0}{\int C_*^{-1}\cdot \exp(-f_{\vb}(\vx_0))\cdot C(\sigma_{\eta-t}^2)^{-1}\cdot \exp\left(-\frac{\left\|\vx-\vx_0\right\|^2}{2\sigma_{\eta-t}^2}\right)\der \vx_0}\\
        & = \E_{\rvx_0 \sim r_{\eta-t|\vb}(\cdot|\vz)}\left[-\frac{\vx-\rvx_0}{\sigma_{\eta-t}^2}\right]
    \end{aligned}
\end{equation*}
and the SDE of $\bkw{\rvx}_t$ to be
\begin{equation*}
    \begin{aligned}
        \der \bkw{\rvx}_t = g^2(\eta - t)\grad \log q_{\eta-t|\vb}(\bkw{\rvx}_t)\der t + g(\eta-t)\der B_t.
    \end{aligned}
\end{equation*}
We can easily obtain that the transition kernel from $\bkw{\rvx}_0$ to  $\bkw{\rvx}_\eta$ is
\begin{equation*}
    \bkw{p}_{\eta|0}(\vx|\vx_0) = C^{-1}(\sigma_\eta^2, \vz_0)\cdot \exp\left(-f_{\vb}(\vx) - \frac{\left\|\vx-\vx_0\right\|^2}{2\sigma_\eta^2}\right),
\end{equation*}
which is introduced for the implementation.

Then, we start to upper bound the contraction of the second stage and have
\begin{equation}
    \label{ineq:kl_contraction_start_stg2}
    \begin{aligned}
        2\partial \KL{\bkw{p}_t}{\bkw{q}_t} &= 2 \int \left(\log \frac{\bkw{p}_t(\vx)}{\bkw{q}_t(\vx)} + 1\right)\cdot \left(\partial_t \bkw{p}_t(\vx)  - \frac{\bkw{p}_t(\vx)}{\bkw{q}_t(\vx)}\cdot \partial_t \bkw{q}_t\right) \der \vx\\
        &\quad + 2 \int \left(\frac{\bkw{p}_t(\vx)}{\bkw{q}_t(\vx)}\log \frac{\bkw{p}_t(\vx)}{\bkw{q}_t(\vx)}\right)\cdot \partial_t \bkw{q}_t(\vx) \der \vx.
    \end{aligned}
\end{equation}
Similar to the analysis in the first stage, we use the Fokker-Planck equation to find the dynamics of the underlying distributions of $\bkw{\rvx}_t$ and $\bkw{\rvz}_t$, which satisfies
\begin{equation*}
    \begin{aligned}
        \partial_t \bkw{p}_t(\vx) & = - \nabla\cdot \left[\bkw{p}_t(\vx) \left(g^2(\eta-t)\grad \log q_{\eta -t|\vb}(\vx)\right)\right] + \Delta \left[\frac{g^2(\eta-t)}{2}\bkw{p}_t(\vx)\right]\\
        & = g^2(\eta - t)\cdot \left(-\nabla\cdot \left(\bkw{p}_t(\vx)\grad \log q_{\eta -t|\vb}(\vx)\right) + \frac{1}{2}\Delta \bkw{p}_t(\vx) \right)\\
        & = g^2(\eta - t)\cdot \left(\nabla \cdot \left(\bkw{p}_t(\vx)\grad \log \frac{\bkw{p}_t(\vx)}{q_{\eta-t|\vb}(\vx)}\right) - \frac{1}{2}\Delta \bkw{p}_t(\vx)\right)\\
        & = g^2(\eta - t)\cdot \left(\nabla \cdot \left(\bkw{p}_t(\vx)\grad \log \frac{\bkw{p}_t(\vx)}{\bkw{q}_{t}(\vx)}\right) + \nabla \cdot \left(\bkw{p}_t(\vx)\grad \log \frac{\bkw{q}_t(\vx)}{\bkw{q}_{t|\vb}(\vx)}\right)  - \frac{1}{2}\Delta \bkw{p}_t(\vx)\right)
    \end{aligned}
\end{equation*}
and 
\begin{equation*}
    \begin{aligned}
        \partial \bkw{q}_t(\vx) &= - \nabla\cdot \left[\bkw{q}_t(\vx) g^2(\eta-t) \grad \log q_{\eta-t}(\vx)\right] +  \Delta\left[\frac{g^2(\eta-t)}{2}\bkw{q}_t(\vx)\right]\\
        & = g^2(\eta - t) \cdot \left(-\nabla \cdot  \left(\bkw{q}_t(\vx)\grad \log q_{\eta - t}(\vx)\right) + \frac{1}{2}\Delta \bkw{q}_t(\vx)\right)\\
        & = g^2(\eta-t) \cdot \left(-\frac{1}{2}\Delta \bkw{q}_t(\vx)\right).
    \end{aligned}
\end{equation*}
Plugging these equations into Eq~\ref{ineq:kl_contraction_start_stg2}, we have
\begin{equation*}
    \begin{aligned}
        2\partial_t \KL{\bkw{p}_t}{\bkw{q}_t} & = g^2(\eta-t) \cdot \int \left(\log \frac{\bkw{p}_t(\vx)}{\bkw{q}_t(\vx)} + 1\right)\cdot \left(2\nabla \cdot \left(\bkw{p}_t(\vx)\grad \log \frac{\bkw{p}_t(\vx)}{\bkw{q}_{t}(\vx)}\right)  -  \Delta \bkw{p}_t(\vx)\right)\der \vx\\
        &\quad + g^2(\eta-t) \cdot \int \left(\log \frac{\bkw{p}_t(\vx)}{\bkw{q}_t(\vx)} + 1\right)\cdot 2 \nabla \cdot \left(\bkw{p}_t(\vx)\grad \log \frac{\bkw{q}_t(\vx)}{\bkw{q}_{t|\vb}(\vx)}\right)\der \vx\\
        &\quad +  g^2(\eta-t) \cdot \int \left(\log \frac{\bkw{p}_t(\vx)}{\bkw{q}_t(\vx)} + 1\right)\cdot\frac{\bkw{p}_t(\vx)}{\bkw{q}_t(\vx)}\cdot \Delta \bkw{q}_t(\vx) \der\vx\\
        &\quad - g^2(\eta-t) \cdot \int \left(\frac{\bkw{p}_t(\vx)}{\bkw{q}_t(\vx)}\log \frac{\bkw{p}_t(\vx)}{\bkw{q}_t(\vx)}\right)\cdot \Delta \bkw{q}_{t}(\vx)\der\vx,
    \end{aligned}
\end{equation*}
which implies
\begin{equation*}
    \begin{aligned}
        2\partial_t \KL{\bkw{p}_t}{\bkw{q}_t} & = \underbrace{2g^2(\eta-t) \cdot \int \left(\log \frac{\bkw{p}_t(\vx)}{\bkw{q}_t(\vx)} + 1\right)\cdot \nabla \cdot \left(\bkw{p}_t(\vx)\grad \log \frac{\bkw{p}_t(\vx)}{\bkw{q}_{t}(\vx)}\right)  \der \vx}_{\mathrm{Term\ 2.1}}\\
        &\quad \underbrace{- g^2(\eta - t)\cdot \left[\int \left(\log \frac{\bkw{p}_t(\vx)}{\bkw{q}_t(\vx)} + 1\right)\cdot \Delta \bkw{p}_t\der \vx +  \int \frac{\bkw{p}_t(\vx)}{\bkw{q}_t(\vx)}\cdot \Delta \bkw{q}_t(\vx)\der\vx\right]}_{\mathrm{Term\ 2.2}}\\
        &\quad \underbrace{+ g^2(\eta-t) \cdot \int \left(\log \frac{\bkw{p}_t(\vx)}{\bkw{q}_t(\vx)} + 1\right)\cdot 2 \nabla \cdot \left(\bkw{p}_t(\vx)\grad \log \frac{\bkw{q}_t(\vx)}{\bkw{q}_{t|\vb}(\vx)}\right)\der \vx}_{\mathrm{Term\ 2.3}}
    \end{aligned}
\end{equation*}
With integration by part and the property of the Laplace operator
\begin{equation*}
    \Delta p(\vx) = \nabla\cdot \left(p(\vx)\grad \log p(\vx)\right),
\end{equation*}

we have
\begin{equation*}
    \mathrm{Term\ 2.1} = -2g^2(\eta - t)\cdot \FI{\bkw{p}_t}{\bkw{q}_t}\quad \mathrm{and}\quad \mathrm{Term\ 2.2} = g^2(\eta - t)\cdot \FI{\bkw{p}_t}{\bkw{q}_t}.
\end{equation*}
Besides, we have
\begin{equation*}
    \begin{aligned}
        \mathrm{Term\ 2.3} & = - 2 g^2(\eta - t) \int \bkw{p}_t(\vx)\left<\grad \log \frac{\bkw{p}_t(\vx)}{\bkw{q}_t(\vx)}, \grad \log \frac{\bkw{q}_t(\vx)}{\bkw{q}_{t|\vb}(\vx)}\right> \der\vx \\
        & \le 2g^2(\eta - t)\int \bkw{p}_t(\vx)\left(\frac{1}{4}\left\|\grad \log \frac{\bkw{p}_t(\vx)}{\bkw{q}_t(\vx)}\right\|^2 + \left\|\grad \log \frac{\bkw{q}_t(\vx)}{\bkw{q}_{t|\vb}(\vx)}\right\|^2\right) \der \vx\\
        & = \frac{g^2(\eta - t)}{2}\FI{\bkw{p}_t}{\bkw{q}_t} + 2g^2(\eta - t)  \int \bkw{p}_t(\vx)\cdot \left\|\grad \log \frac{\bkw{q}_t(\vx)}{\bkw{q}_{t|\vb}(\vx)}\right\|^2 \der \vx.
    \end{aligned}
\end{equation*}
For the last term, we have
\begin{equation*}
    \begin{aligned}
        \left\|\grad \log \frac{\bkw{q}_t(\vx)}{\bkw{q}_{t|\vb}(\vx)}\right\|^2 = \left\|\sigma_{\eta-t}^{-2}\cdot \left(\E_{\rvx_0\sim r_{\eta-t|\vb}(\cdot|\vx)}\left[\rvx_0\right] - \E_{\rvx_0\sim r_{\eta-t}(\cdot|\vx)}\left[\rvx_0\right]\right)\right\|^2
    \end{aligned}
\end{equation*}
which follows from Eq~\ref{ineq:score_formula}.
Essentially, we require
\begin{equation*}
    \int_0^{\eta} \frac{g^2(\eta-t)}{\left(\int_0^{\eta-t}g^2(s)\der s\right)^2}\der t = \mathcal{O}(1).
\end{equation*}
