# Supplementary material for: Faster Sampling via Stochastic Gradient Proximal Sampler
Source: arXiv:2405.16734 source file (2024-05-27)
Supplement: Supplementary file 2 [file 05Lem_CompStage2.tex]

\section{The Composite Second Stage}

Inheriting notations presented in Section~\ref{sec:not_ass_0x},
since we only consider one update of $\rvx_k$,  we abbreviate $\rvx_k$ and $\rvx_{k+1/2}$ as $\rvx_0$ and $\rvx_\eta$ for simplification. 
For the second stage, the random variables $\rvx_{k+1/2}$ and $\rvx_{k+1}$ abbreviated as $\rbkwx_0$ and $\rbkwx_\eta$.

The same abbreviation is also used for $\tilde{\rvx}_k$, $\tilde{\rvx}_{k+1/2}$, $\tilde{\rvx}_{k+1}$, and we have
\begin{equation*}
    \tilde{\rvx}_0 \coloneqq \tilde{\rvx}_k, \quad \bkw{\tilde{\rvx}}_0 = \tilde{\rvx}_\eta \coloneqq \tilde{\rvx}_{k+\frac{1}{2}}\quad \mathrm{and}\quad \bkw{\tilde{\rvx}}_\eta \coloneqq \tilde{\rvx}_{k+1}.
\end{equation*}
As its definition shown in Eq~\ref{def:transition_kernel_fullgrad}, it has
\begin{equation*}
    \begin{aligned}
        &\tilde{p}_{\eta|0}(\vx^\prime|\vx) = C(\eta)^{-1}\cdot \exp\left(-\frac{\left\|\vx^\prime - \vx\right\|^2}{2\eta}\right)\\
        &\bkw{\tilde{p}}_{\eta|0}(\vx^\prime|\vx) = C(\eta,\vx)^{-1}\cdot \exp\left(-f(\vx^\prime)-\frac{\left\|\vx^\prime - \vx\right\|^2}{2\eta}\right).
    \end{aligned}
\end{equation*}
An important property of these random variables is $\bkw{\tilde{p}}_\eta \propto \exp(-f)$ when $\tilde{p}_0 \propto \exp(-f)$.
In this condition, we want to extend them to two Markov processes $\{\tilde{\rvx}_t\}_{t\in[0,\eta]}$ and $\{\bkw{\tilde{\rvx}}_t\}_{t\in[0,\eta]}$ which satisfies $\tilde{\rvx}_t = \bkw{\tilde{\rvx}}_{\eta - t}$.
A concise construction requires
\begin{equation*}
    \der \tilde{\rvx}_t = \der B_t
\end{equation*}
and consider $\{\bkw{\tilde{\rvx}}_t\}_{t\in[0,\eta]}$ as its reverse SDE, i.e.,
\begin{equation*}
    \der \bkw{\tilde{\rvx}}_t = \grad \log \tilde{p}_{\eta-t}(\rbkwx_t)+\der B_t.
\end{equation*}

To investigate the convergence for any batch size, we try to consider the transition kernel from $\bkw{\tilde{\rvx}}_{t_0}$ to $\bkw{\tilde{\rvx}}_{t}$ where $t_0< t$. 
Considering the general transition kernel $\bkw{\tilde{p}}_{t|t_0}(\vx|\vx_0)$ as 
\begin{equation}
    \label{eq:condi_TransKer_general}
    \bkw{\tilde{p}}_{t|t_0}(\vx|\vx_0) = \left(\bkw{\tilde{p}}_{\eta-t_0|0}(\cdot|\vx_0) \ast \varphi_{\eta - t}\right)(\vx),
\end{equation}
which can be validated by checking the establishment of the equation
\begin{equation*}
    \bkw{\tilde{p}}_t(\vx) = \int \bkw{\tilde{p}}_{t_0}(\vx_0) \bkw{\tilde{p}}_{t|t_0}(\vx|\vx_0) \der \vx_0.
\end{equation*}
For the LHS, we have
\begin{equation*}
    \begin{aligned}
        \bkw{\tilde{p}}_t(\vx) = \tilde{p}_{\eta - t}(\vx) = \int C_0^{-1}\cdot \exp(-f(\vx_0))\cdot C^{-1}_{\vx,\eta-t}\cdot\exp\left(-\frac{\left\|\vx-\vx_0\right\|^2}{2(\eta-t)}\right)\der \vx_0.
    \end{aligned}
\end{equation*}
For the RHS, we have
\begin{equation*}
    \scriptstyle
    \begin{aligned}
        &\int \bkw{\tilde{p}}_{t_0}(\vx_0) \bkw{\tilde{p}}_{t|t_0}(\vx|\bkwx_0) \der \vx_0 \\
        &= \int \bkw{\tilde{p}}_{t_0}(\vx_0) \cdot \left(\int C_{\vx_0,\eta-t_0}^{-1}\exp\left(-f(\vx_2)-\frac{\left\|\vx_2-\vx_0\right\|^2}{2(\eta - t_0)}\right)\cdot C^{-1}_{\vx,\eta-t}\cdot \exp\left(-\frac{\left\|\vx-\vx_2\right\|^2}{2(\eta-t)}\right) \der \vx_2\right) \der \vx_0\\
        &= \int C^{-1}_{\vx,\eta-t}\cdot \exp\left(-\frac{\left\|\vx-\vx_2\right\|^2}{2(\eta-t)}\right)\cdot \underbrace{\left(\int \bkw{\tilde{p}}_{t_0}(\vx_0)\cdot C_{\vx_0,\eta-t_0}^{-1}\exp\left(-f(\vx_2)-\frac{\left\|\vx_2-\vx_0\right\|^2}{2(\eta - t_0)}\right)\der\vx_0\right)}_{\text{Term 2.1}}\der \vx_2.
    \end{aligned}
\end{equation*}
In addition, we have $\mathrm{Term\ 2.1}=C_*^{-1}\exp(-f(\vx_2))$ since we have
\begin{equation*}
    \begin{aligned}
        \mathrm{Term\ 2.1} & = \int \tilde{p}_{\eta - t_0}(\vx_0)\cdot C_{\vx_0,\eta-t_0}^{-1}\exp\left(-f(\vx_2)-\frac{\left\|\vx_2-\vx_0\right\|^2}{2(\eta - t_0)}\right)\der\vx_0\\
        & = \int \left(\int C_*^{-1}\cdot C_{(\eta - t_0)}^{-1}\cdot \exp\left(-f(\vx^\prime)-\frac{\left\|\vx_0-\vx^\prime\right\|^2}{2(\eta - t_0)}\right)\der \vx^\prime\right) \cdot C_{\vx_0,\eta-t_0}^{-1}\exp\left(-f(\vx_2)-\frac{\left\|\vx_2-\vx_0\right\|^2}{2(\eta - t_0)}\right)\der\vx_0\\
        & = C_*^{-1}\exp(-f(\vx_2))\cdot \int \left(\int C_{\vx_0, \eta - t_0}^{-1}\cdot \exp\left(-f(\vx^\prime)- \frac{\left\|\vx_0-\vx^\prime\right\|^2}{2(\eta-t_0)}\right)\der \vx^\prime\right) C_{\eta-t_0}^{-1}\cdot \exp\left(-\frac{\left\|\vx_2-\vx_0\right\|^2}{2(\eta - t_0)}\right)\der \vx_0\\
        & = C_*^{-1}\exp(-f(\vx_2)).
    \end{aligned}
\end{equation*}

We divide the second stage into several sub-stages, which correspond to the transitions among $(\bkw{\tilde{\rvx}}_0, \bkw{\tilde{\rvx}}_\tau, \ldots, \bkw{\tilde{\rvx}}_{S\tau})$ where $S\in \mathbb{N}_+$ and $S\tau = \eta$.
Hence, we introduce a variant stochastic proximal sampler.
\begin{algorithm}[!htbp]
    \caption{Stochastic Proximal Sampler}
    \label{alg:sps_var}
    \begin{algorithmic}[1]
            \State {\bfseries Input:} The negative log density $f$ of the target distribution, the initial particle $\vx_0$ drawn from $p_0$;
            \For{$k=1$ to $K$}
                \State Draw the sample $\vx_{k+1/2}$ from $\mathcal{N}(\vx_k, \eta\mI)$;
                \State Initial the particle of the inner loop as $\bkw{\vx}_0\gets \vx_{k+1/2}$;
                \For {$s=1$ to $S$}
                    \State Draw the mini-batch $\vb_{s}$ from $\{1,2,\ldots, n\}$;
                    \State Draw the sample $\bkw{\vx}_{s\tau}$ from  $\bkw{p}_{s\tau|(s-1)\tau,b}(\cdot|\vx_{(s-1)\tau},\vb_s)$;
                \EndFor
                \State Set $\vx_{k+1}\gets \bkw{\vx}_{S\tau}$;
            \EndFor
            \State {\bfseries Return:} $\vx_{K+1}$.          
    \end{algorithmic}
\end{algorithm}

In Alg~\ref{alg:sps_var}, we should note the implementation of Line 7.
Specifically, with Eq~\ref{eq:condi_TransKer_general}, we have $\bkw{\tilde{p}}_{t|t_0}(\vx|\vx_0) = \left(\bkw{\tilde{p}}_{\eta-t_0|0}(\cdot|\vx_0) \ast \varphi_{\eta - t}\right)(\vx)$, which means a particle $\bkw{\tilde{\rvx}}_{s\tau}$ sampling from $\bkw{\tilde{p}}_{s\tau|(s-1)\tau}(\cdot|\vx_{(s-1)\tau})$ can be presented as a sum of two random variables $\bkw{\tilde{\rvz}}_{s\tau}$ and $\xi_{s\tau}$ satisfying
\begin{equation*}
    \begin{aligned}
        &\bkw{\tilde{\rvz}}_{s\tau}\sim \bkw{\tilde{p}}_{\eta - (s-1)\tau|0}(\cdot|\vx_{(s-1)\tau}) = C(\eta-(s-1)\tau,\vx_{(s-1)\tau})^{-1}\cdot \exp\left(-f(\cdot) - \frac{\left\|\cdot - \vx_{(s-1)\tau}\right\|^2}{2(\eta-(s-1)\tau)}\right)\\
        &\xi_{st} \sim \mathcal{N}(\vzero, (\eta-s\tau)\cdot \mI).  
    \end{aligned}
\end{equation*}
Extend it to the randomized version, requiring a particle $\bkw{\rvx}_{s\tau}$ from $\bkw{p}_{s\tau|(s-1)\tau,b}(\cdot|\vx_{(s-1)\tau},\vb_s)$, we have the presentation $\bkw{\rvx}_{s\tau} = \bkw{\rvz}_{s\tau} + \xi_{s\tau}$ which satisfies
\begin{equation*}
    \begin{aligned}
        &\bkw{\rvz}_{s\tau}\sim \bkw{p}_{\eta - (s-1)\tau|0,b}(\cdot|\vx_{(s-1)\tau}, \vb_s) = C(\vb_s,\eta-(s-1)\tau,\vx_{(s-1)\tau})^{-1}\cdot \exp\left(-f_{\vb_s}(\cdot) - \frac{\left\|\cdot - \vx_{(s-1)\tau}\right\|^2}{2(\eta-(s-1)\tau)}\right)\\
        &\xi_{st} \sim \mathcal{N}(\vzero, (\eta-s\tau)\cdot \mI).  
    \end{aligned}
\end{equation*}
In this condition, we only consider the contraction of the last iteration and have
\begin{equation*}
    \begin{aligned}
        \KL{\tilde{p}_{K+1}}{p_{K+1}} &= \KL{\bkw{\tilde{p}}_{S\tau}}{\bkw{p}_{S\tau}} \le \KL{\bkw{\tilde{p}}_{S\tau, (S-1)\tau, b}}{\bkw{p}_{S\tau, (S-1)\tau, b}}\\
        &\le \KL{\bkw{\tilde{p}}_{(S-1)\tau}}{\bkw{p}_{(S-1)\tau}} + \E_{(\rvx, \rvb)\sim \bkw{\tilde{p}}_{(S-1)\tau, b}}\left[\KL{\bkw{\tilde{p}}_{S\tau|(S-1)\tau, b}(\cdot|\rvx,\rvb)}{\bkw{p}_{S\tau|(S-1)\tau, b}(\cdot|\rvx,\rvb)}\right]
    \end{aligned}
\end{equation*}
