# Supplementary material for: Faster Sampling via Stochastic Gradient Proximal Sampler
Source: arXiv:2405.16734 source file (2024-05-27)
Supplement: Supplementary file 3 [file backup.tex]

\section{Analysis}
We first consider the SDE and transition kernels in each two-stage update of proximal samplers~\cite{chen2022improved}.
In the following, we only consider one iteration.
At the $k$-th update, the first stage's underlying distribution at time $t$ is denoted as $\tilde{p}_{(k,1),t}$, and $\tilde{p}_{(k,2),t}$ presents the underlying distribution at time $t$ in the second stage.
We have $\tilde{p}_{(k,1), \eta} = \tilde{p}_{(k,2),0}$.
\paragraph{Stage 1.} 
The transition kernel of the stage 1 is
\begin{equation*}
    \tilde{p}_{(k,1),\eta|0}(\vx|\vx_0) = \left(2\pi \eta\right)^{-d/2}\cdot \exp\left(-\frac{1}{2}\cdot \frac{\left\|\vx-\vx_0\right\|^2}{\eta}\right)\coloneqq C_\eta^{-1}\cdot \exp\left(-\frac{1}{2}\cdot \frac{\left\|\vx-\vx_0\right\|^2}{\eta}\right).
\end{equation*}
This transition kernel corresponds to the following SDE
\begin{equation}
    \label{sde:first_stage}
    \der \tilde{\rvx}_{(k,1),t} = \der B_t.
\end{equation}
Suppose we have $\tilde{p}_{(k,1), 0}=C_0^{-1}\cdot \exp(-f)$, then the underlying distribution of $\tilde{p}_{(k,1),\eta}$ is
\begin{equation}
    \label{ineq:tar_den_half}
    \begin{aligned}
        \tilde{p}_{(k,1), \eta}(\vx) = & \int \tilde{p}_{(k,1),0}(\vx_0) \tilde{p}_{(k,1),\eta|0}(\vx|\vx_0)\der\vx_0\\
        = & \int C_0^{-1}\cdot \exp\left(-f(\vx_0)\right)\cdot C_\eta^{-1}\cdot \exp\left(-\frac{\left\|\vx-\vx_0\right\|^2}{2\eta}\right)\der \vx_0\\
        = & C_0^{-1}C_\eta^{-1}\cdot \int \exp\left(-f(\vx_0)-\frac{\left\|\vx-\vx_0\right\|^2}{2\eta}\right)\der \vx_0
    \end{aligned}
\end{equation}
\paragraph{Stage 2.} In this stage, we only know its transition kernel, i.e.,
\begin{equation*}
    \begin{aligned}
        \tilde{p}_{(k,2),\eta|0}(\vx|\vx_0) = C_1^{-1}(\vx_0)\exp\left(-f(\vx)-\frac{\left\|\vx-\vx_0\right\|^2}{2\eta}\right) 
    \end{aligned}
\end{equation*}
and expect to find some interpolating SDE corresponding to such a kernel. 
Supposing $\tilde{p}_{(k,2),0} = \tilde{p}_{(k,1),\eta}$ shown in Eq~\ref{ineq:tar_den_half}, then we have
\begin{equation}
    \label{eq:tar_den_wh}
    \begin{aligned}
        \tilde{p}_{(k,2),\eta}(\vx) = & \int \tilde{p}_{(k,2),0}(\vx_0)\tilde{p}_{(k,2),\eta|0}(\vx|\vx_0)\der \vx_0\\
        = & \int_{\vx_0} \left[C_0^{-1}C_\eta^{-1}\cdot \int_{\vx^\prime} \exp \left(-f(\vx^\prime)-\frac{\left\|\vx_0-\vx^\prime\right\|^2}{2\eta}\right)\der \vx^\prime \cdot C_1(\vx_0)^{-1}\cdot \exp\left(-f(\vx)-\frac{\left\|\vx-\vx_0\right\|^2}{2\eta}\right)\right]\der\vx_0\\
        = & C_0^{-1}\exp\left(-f(\vx)\right)\cdot \int_{\vx_0} \left[\underbrace{C_1(\vx_0)^{-1}\int_{\vx^\prime}\exp\left(-f(\vx^\prime) -\frac{\left\|\vx_0-\vx^\prime\right\|^2}{2\eta}\right)\der \vx^\prime}_{\text{Term 1}}\right]\cdot C_\eta^{-1}\exp\left(\frac{-\left\|\vx-\vx_0\right\|^2}{2\eta}\right)\der \vx_0
    \end{aligned}
\end{equation}
It can be easily observed that $\mathrm{Term\ 1} = 1$, and for any $\vx_0,\vx_1\in\R^d$, it has
\begin{equation*}
    \begin{aligned}
        \int \exp\left(-\frac{\left\|\vx-\vx_0\right\|^2}{2\eta}\right) \der\vx = \int \exp\left(-\frac{\left\|\vx-\vx_1\right\|^2}{2\eta}\right) \der\vx = C_\eta,
    \end{aligned}
\end{equation*}
which mean Eq~\ref{eq:tar_den_wh} can be rewritten as
\begin{equation*}
    \begin{aligned}
        \tilde{p}_{(k,2),\eta}(\vx) = C_0^{-1}\exp(-f(\vx))\cdot \int_{\vx_0} C_\eta^{-1}\exp\left(\frac{-\left\|\vx-\vx_0\right\|^2}{2\eta}\right)\der \vx_0 = C_0^{-1}\exp(-f(\vx)).
    \end{aligned}
\end{equation*}
It means $\exp(-f(\vx))$ is the stationary distribution under such a two-stage update, \textcolor{blue}{and the introplating SDE of the second stage can be considered as the reverse SDE of the first one when its initialized with $\exp(-f)$}.
According to~\cite{chen2022sampling}, the reverse SDE of SDE~\ref{sde:first_stage} is 
\begin{equation}
    \label{sde:second_stage}
    \der \tilde{\rvx}_{(k,2),t} = \grad \log \tilde{p}_{(k,1), T-t}(\tilde{\rvx}_{(k,2),t}) \der t + \der B_t,
\end{equation}
where $\tilde{p}_{(k,1),t}$ is the density function of the forward process and can be written as
\begin{equation*}
    \begin{aligned}
        \tilde{p}_{(k,1),t}(\vx) = & \int \tilde{p}_{(k,1),0} (\vx_0)\tilde{p}_{(k,1),t|0}(\vx|\vx_0)\der \vx_0\\
        = & \int C_0^{-1}\exp(-f(\vx_0))\cdot C_t^{-1}\cdot \exp\left(-\frac{\left\|\vx-\vx_0\right\|^2}{2t}\right) \der \vx_0,
    \end{aligned}
\end{equation*}
which is similar to Eq~\ref{ineq:tar_den_half}.
Therefore, we have
\begin{equation*}
    \begin{aligned}
        \grad \ln \tilde{p}_{(k,1),t}(\vx) = &\frac{\grad \tilde{p}_{(k,1),t}(\vx)}{\tilde{p}_{(k,1),t}(\vx)} = \frac{\int C_0^{-1}\exp(-f(\vx_0))\cdot C_t^{-1}\cdot \exp\left(-\frac{\left\|\vx-\vx_0\right\|^2}{2t}\right)\cdot \left(-\frac{\vx-\vx_0}{t}\right) \der \vx_0}{\int C_0^{-1}\exp(-f(\vx_0))\cdot C_t^{-1}\cdot \exp\left(-\frac{\left\|\vx-\vx_0\right\|^2}{2t}\right) \der \vx_0}\\
        = & \E_{\rvx_0\sim \tilde{q}_{t}(\cdot|\vx)}\left[-\frac{\vx - \rvx_0}{t}\right]
    \end{aligned}
\end{equation*}
where $\tilde{q}_t(\cdot|\vx)$ can be written as
\begin{equation*}
    \begin{aligned}
        \tilde{q}_t(\vx_0|\vx) \propto \exp\left(-f(\vx_0)-\frac{\left\|\vx-\vx_0\right\|^2}{2t}\right).
    \end{aligned}
\end{equation*}
With this condition, we can rewrite SDE~\ref{sde:second_stage} as
\begin{equation}
    \label{sde:second_stage_fin}
    \der \tilde{\rvx}_{(k,2),t} = \left(-\frac{\tilde{\rvx}_{(k,2),t}}{T-t} + \frac{\E_{\rvx^\prime \sim q_{T-t}(\cdot|\tilde{\rvx}_{(k,2),t})}[\rvx^\prime]}{T-t} \right) \der t + \der B_t.
\end{equation}
We should note that this SDE is only equivalent to the update when the timestamp is $\eta$, which is why we call it intropolating SDE. 
This methodology is also used in our analysis of dimension-free ULA.

\section{Implementation of stochastic proximal samplers}
\begin{algorithm}[!htbp]
    \caption{Stochastic Proximal Sampler}
    \label{alg:sps}
    \begin{algorithmic}[1]
            \State {\bfseries Input:} The negative log density $f$ of the target distribution, the initial particle $\vx_0$ drawn from $p_0$;
            \For{$k=0$ to $K-1$}
                \State Draw the sample $\vx_{k+1/2}$ from $\mathcal{N}(\vx_k, \eta\mI)$;
                \State Draw the mini-batch $\vb$ from $\{1,2,\ldots, N\}$;
                \State Draw the sample $\vx_{k+1}$ from  $\bkwp(\cdot|\vx_{k+1/2},\vb)$;
            \EndFor
            \State {\bfseries Return:} $\vx_{K}$.
    \end{algorithmic}
\end{algorithm}
To control the KL divergence gap of the output particles' underlying distributions between the proximal sampler and its randomized version.
We consider the following two-stage update
\begin{itemize}
    \item The update of the first stage follows from the SDE:
        \begin{equation}
            \label{sde:first_stage_prac}
            \der \rvx_{(k,1),t} = \der B_t,
        \end{equation}
        which is the same as that in the deterministic version since it does not require any gradient oracles.
    \item The update of the second stage when the mini-batch is given follows from the SDE:
        \begin{equation}
            \begin{aligned}
            \label{sde:second_stage_prac}
            \der \rvx_{(k,2),t} = &\grad\log p_{(k,1),T-t}(\rvx_{(k,2),t},\vb)\der t + \der B_t \\
            \coloneqq &\left(-\frac{\rvx_{(k,2),t}}{T-t} + \frac{\E_{\rvx^\prime \sim q_{T-t}(\cdot|\rvx_{(k,2),t},\vb)}[\rvx^\prime]}{T-t} \right) \der t + \der B_t,
            \end{aligned}
        \end{equation}
        where $q_{T-t}(\cdot|\vx,\vb)$ denotes
        \begin{equation}
            \label{sde:second_stage_prac_q}
            q_{T-t}(\vx^\prime|\vx,\vb) \propto \exp\left(-f_{\vb}(\vx^\prime) - \frac{\left\|\vx^\prime-\vx\right\|^2}{2(T-t)}\right)
        \end{equation}
        and $f_{\vb}$ denotes the mini-batch loss.
\end{itemize}
With the same techniques utilized in the previous section, we can provide a specific transition kernel for the implementation of the second stage, i.e.,
\begin{equation*}
    \begin{aligned}
        p_{(k,2),\eta|0}(\vx|\vx_0, \vb) \propto \exp\left(-f_{\vb}(\vx)-\frac{\left\|\vx-\vx_0\right\|^2}{2\eta}\right) 
    \end{aligned}
\end{equation*}

In this condition, we can implement it with the following algorithm, i.e., Alg~\ref{alg:sps}


\paragraph{Control the gap between the standard SDE and the stochastic version with Girsanov Theorem~\cite{chen2023improved}.}
We show the intuition of our analysis by illustrating the two SDEs in Fig~\ref{fig:sps}.
\begin{figure}[!hbpt]
        \centering
        \resizebox{0.7\textwidth}{!}{%
        \input{0_figs/sps_explain}
        }
        \caption{Illustration of SPS.}
        \label{fig:sps}
\end{figure}

\textcolor{red}{The key point is utilized the introplating SDE and Girsanov Theorem rather than the transition kernel. We expect to obtain a stochastic sampling algorithm with better gradient complexity (for the $\epsilon$ order).}

\paragraph{Proof Roadmap.} To use the triangle inequality, we first consider the convergence of total variation distance.
\begin{equation*}
    \begin{aligned}
        \TVD{p_{(K,2),\eta}}{p_*}^2 \le & 2\TVD{p_{(K,2),\eta}}{\tilde{p}_{(K,2),\eta}}^2 + 2\TVD{\tilde{p}_{(K,2),\eta}}{p_*}^2\\
        \le & \underbrace{\KL{\tilde{p}_{(K,2),\eta}}{p_{(K,2),\eta}}}_{\mathrm{Term\ 1}} + \underbrace{\KL{\tilde{p}_{(K,2),\eta}}{p_*}}_{\mathrm{Term\ 2}}.
    \end{aligned}
\end{equation*}
To upper bound Term 2, we introduce the standard analysis of proximal samplers shown in~\cite{chen2022improved}.

As for Term 1, we can use the similar idea as that in~\cite{chen2023improved}.
Specifically, consider the following two SDEs of the second stage, i.e.,
\begin{equation}
    \label{sde:second_stage_ite}
    \der \tilde{\rvx}_{(k,2),t} = \left(-\frac{\tilde{\rvx}_{(k,2),t}}{T-t} + \frac{\E_{\rvx^\prime \sim q_{T-t}(\cdot|\tilde{\rvx}_{(k,2),t})}[\rvx^\prime]}{T-t} \right) \der t + \der B_t,\quad \tilde{\rvx}_{(k,2),0} = \vx_0\ \mathrm{and}\ \tilde{\rvb} = \vb.  
\end{equation}
and
\begin{equation}
    \label{sde:second_stage_prac_ite}
    \der \rvx_{(k,2),t} = \left(-\frac{\rvx_{(k,2),t}}{T-t} + \frac{\E_{\rvx^\prime \sim q_{T-t}(\cdot|\rvx_{(k,2),t},\vb)}[\rvx^\prime]}{T-t} \right) \der t + \der B_t,\quad \rvx_{(k,2),0}=\vx_0\ \mathrm{and}\ \rvb=\vb.
\end{equation}
According to Lemma 6 of~\cite{chen2023improved}, we have
\begin{equation*}
    \begin{aligned}
        &\frac{\partial}{\partial t}\KL{\tilde{p}_{(k,2),t}}{p_{(k,2),t}} = -\FI{\tilde{p}_{(k,2),t}}{p_{(k,2),t}} \\
        &\quad + (T-t)^{-1}\cdot \E_{\tilde{\rvx}\sim \tilde{p}_{(k,2),t}}\left[\left<\E_{\rvx^\prime \sim q_{T-t}(\cdot|\tilde{\rvx})}[\rvx^\prime]-\E_{\rvx^\prime \sim q_{T-t}(\cdot|\tilde{\rvx},\vb)}[\rvx^\prime], \grad \log \frac{\tilde{p}_t^{(2)}(\tilde{\rvx})}{p_t^{(2)}(\tilde{\rvx})}\right>\right]\\
        &\le (2T-2t)^{-2} \cdot \E_{\tilde{\rvx}\sim \tilde{p}_{(k,2),t}}\left[\left\|\E_{\rvx^\prime \sim q_{T-t}(\cdot|\tilde{\rvx})}[\rvx^\prime]-\E_{\rvx^\prime \sim q_{T-t}(\cdot|\tilde{\rvx},\vb)}[\rvx^\prime]\right\|^2\right].
    \end{aligned}
\end{equation*}
It can be easily noted that the integration of the upper bound will be divergent. 
We consider another proof roadmap.

\section{Introducing the shrinking SDE}
We consider two shrinking versions of deterministic and stochastic SDEs.

The shrinking version of the deterministic proximal sampler also has a two-stage update. 
The update of stage 1 is
\begin{equation*}
    \underline{\tilde{p}}_{(k,1),(\eta-(k-1)\Delta)|0} (\vx|\vx_0)= \left(2\pi \cdot (\eta - (k-1)\Delta)\right)^{-d/2}\cdot \exp\left(-\frac{1}{2}\cdot \frac{\left\|\vx-\vx_0\right\|^2}{\eta - (k-1)\Delta}\right).
\end{equation*}
Suppose we have
\begin{equation*}
    g_*(\vx)\coloneqq \exp(-f(\vx))\quad \mathrm{and}\quad \varphi_{k\Delta}\coloneqq \exp\left(-\frac{1}{2}\cdot \frac{\left\|\vx\right\|^2}{k\Delta}\right)
\end{equation*}
the update of stage 2 is
\begin{equation*}
    \underline{\tilde{p}}_{(k,2),(\eta-k\Delta)}(\vx|\vx_0) = C_2^{-1}(\vx_0,k)\cdot \left(g_* \ast \varphi_{k\Delta}\right)(\vx)\cdot  \exp\left(-\frac{\left\|\vx-\vx_0\right\|^2}{2(\eta - k\Delta)}\right).
\end{equation*}
We should note that for the update of stage 2, there exists another formulation that can be proved to be equivalent to the above conditional probability.
\begin{equation*}
    \begin{aligned}
        \underline{\tilde{p}}_{(k,2),(\eta-k\Delta)}(\vx|\vx_0) = & C_1^{-1}(\vx_0, k)\int \exp\left(-f(\vy)-\frac{\left\|\vy-\vx_0\right\|^2}{2\eta}\right)\cdot \exp\left(-\frac{\left\|\vx-\vy\right\|^2}{k\Delta}\right)\der \vy\\
        = & C_1^{-1}(\vx_0, k)
    \end{aligned}
\end{equation*}

We also consider the shrinking version of the stochastic proximal sampler, whose two-stage update is 
\begin{equation*}
    \underline{p}_{(k,1),(\eta-(k-1)\Delta)|0} (\vx|\vx_0)= \left(2\pi \cdot (\eta - (k-1)\Delta)\right)^{-d/2}\cdot \exp\left(-\frac{1}{2}\cdot \frac{\left\|\vx-\vx_0\right\|^2}{\eta - (k-1)\Delta}\right),
\end{equation*}
and
\begin{equation*}
    \underline{p}_{(k,2),(\eta-k\Delta)}(\vx|\vx_0) = C_1^{-1}(\vx_0,k)\cdot \left(g_{*,\vb} \ast \varphi_{k\Delta}\right)(\vx)\cdot  \exp\left(-\frac{\left\|\vx-\vx_0\right\|^2}{2(\eta - k\Delta)}\right),
\end{equation*}
\textcolor{red}{Maybe, we can use another formulation to put the convolution outside.}
where 
\begin{equation*}
    g_{*\vb}(\vx)\coloneqq \exp(-f_{\vb}(\vx)).
\end{equation*}

In the following, we suppose that $p_{(1,1),0}$ and $\underline{p}_{(1,1),0}$ are the same and set as a Gaussian distribution.
Besides, $\tilde{p}_{(1,1),0}$ and $\underline{\tilde{p}}_{(1,1),0}$ are set as $p_*$.
We have the following bound
\begin{equation*}
    \begin{aligned}
        \TVD{p_{(K,2),\eta}}{p_*} \le & \TVD{p_{(K,2),\eta}}{\underline{p}_{(K,2),\eta-K\Delta}}+\TVD{\underline{p}_{(K,2),\eta-K\Delta}}{p_*}\\
        \le & \underbrace{\TVD{p_{(K,2),\eta}}{\underline{p}_{(K,2),\eta-K\Delta}}}_{\text{Term 1}}+ \underbrace{\TVD{\underline{p}_{(K,2),\eta-K\Delta}}{\underline{\tilde{p}}_{(K,2),\eta-K\Delta}}}_{\text{Term 2}}+\underbrace{\TVD{\underline{\tilde{p}}_{(K,2),\eta-K\Delta}}{\tilde{p}_{(K,2),\eta}}}_{\text{Term 3}}.
    \end{aligned}
\end{equation*}
\paragraph{Upper bound Term 1.}
According to Pinsker's inequality, we have
\begin{equation*}
    \TVD{p_{(K,2),\eta}}{\underline{p}_{(K,2),\eta-K\Delta}} \le \sqrt{\frac{1}{2}\KL{\underline{p}_{(K,2),\eta-K\Delta}}{p_{(K,2),\eta}}}
\end{equation*}
and we upper bound the KL divergence in the following.
Due to the following inequality, 
\begin{equation}
    \label{ineq:end_kl_ubp}
    \small
    \begin{aligned}
        &\KL{\underline{p}_{(K,2),(\eta-K\Delta,0,b)}}{p_{(K,2),(\eta,0,b)}}=\int \underline{p}_{(K,2),(\eta-K\Delta,0,b)}(\vx,\vx_0,\vb)\log \frac{\underline{p}_{(K,2),(\eta-K\Delta,0,b)}(\vx,\vx_0,\vb)}{p_{(K,2),(\eta,0,b)}(\vx,\vx_0,\vb)}  \der (\vx,\vx_0,\vb)\\
        &\quad = \int \underline{p}_{(K,2),(\eta-K\Delta,0,b)}(\vx,\vx_0,\vb)\left(\log \frac{\underline{p}_{(K,2),(0,b|\eta-K\Delta)}(\vx_0,\vb|\vx)}{p_{(K,2),(0,b|\eta)}(\vx_0,\vb|\vx)}+\log\frac{\underline{p}_{(K,2),(\eta-K\Delta)}(\vx)}{p_{(K,2),\eta}(\vx)}\right)  \der (\vx,\vx_0,\vb)\\
        &\quad =\E_{\rvx\sim\underline{p}_{(K-2),\eta}}\left[\KL{\underline{p}_{(K,2),(0,b|\eta-K\Delta)}(\cdot|\rvx)}{p_{(K,2),(0,b|\eta)}(\cdot|\rvx)}\right] + \KL{\underline{p}_{(K,2),\eta-K\Delta}}{p_{(K,2),\eta}}\\
        &\quad \ge \KL{\underline{p}_{(K,2),\eta-K\Delta}}{p_{(K,2),\eta}}.
    \end{aligned}
\end{equation}
With the same technique, we have
\begin{equation}
    \label{eq:comb_kl}
    \small
    \begin{aligned}
        &\KL{\underline{p}_{(K,2),(\eta-K\Delta,0,b)}}{p_{(K,2),(\eta,0,b)}} \le \KL{\underline{p}_{(K,2),0}}{p_{(K,2),0}}+\E_{\rvx_0\sim \underline{p}_{(K,2),0}}\left[\KL{\underline{p}_{(K,2),(b|0)}(\cdot|\rvx_0)}{p_{(K,2),(b|0)}(\cdot|\rvx_0)}\right]\\
        &\quad +\E_{(\rvx_0,\rvb)\sim \underline{p}_{(K,2),(0,b)}}\left[\KL{\underline{p}_{(K,2),(\eta-K\Delta|0,b)}(\cdot|\rvx_0,\rvb)}{p_{(K,2),(\eta|0,b)}(\cdot|\rvx_0,\rvb)}\right].
    \end{aligned}
\end{equation}
Combining Eq~\ref{ineq:end_kl_ubp} and Eq~\ref{eq:comb_kl}, we have
\begin{equation}
    \small
    \label{ineq:term1_mid}
    \begin{aligned}
        &\KL{\underline{p}_{(K,2),\eta-K\Delta}}{p_{(K,2),\eta}} \le \KL{\underline{p}_{(K,2),0}}{p_{(K,2),0}}+\E_{\rvx_0\sim \underline{p}_{(K,2),0}}\left[\KL{\underline{p}_{(K,2),(b|0)}(\cdot|\rvx_0)}{p_{(K,2),(b|0)}(\cdot|\rvx_0)}\right]\\
        &\quad +\E_{(\rvx_0,\rvb)\sim \underline{p}_{(K,2),(0,b)}}\left[\KL{\underline{p}_{(K,2),(\eta-K\Delta|0,b)}(\cdot|\rvx_0,\rvb)}{p_{(K,2),(\eta|0,b)}(\cdot|\rvx_0,\rvb)}\right]\\
        & =\underbrace{\KL{\underline{p}_{(K,2),0}}{p_{(K,2),0}}}_{\text{Term 1.1}} +\underbrace{\E_{(\rvx_0,\rvb)\sim \underline{p}_{(K,2),(0,b)}}\left[\KL{\underline{p}_{(K,2),(\eta-K\Delta|0,b)}(\cdot|\rvx_0,\rvb)}{p_{(K,2),(\eta|0,b)}(\cdot|\rvx_0,\rvb)}\right]}_{\text{Term 1.2}}.
    \end{aligned}
\end{equation}
where the last equation establishes by requiring 
\begin{equation*}
    \underline{p}_{(K,2), (b|0)}(\cdot|\vx) = p_{(K,2), (b|0)}(\cdot|\vx)\quad \forall\ \vx\in\R^d.
\end{equation*}
This condition is obviously true due to the mini-batch $\rvb$ is independent with $\rvx_{(K,2),0}$.
Then, we need to upper bound Term 1.2, for any $\rvx_0 =\vx$ and $\rvb = \vb$, we consider
\begin{equation*}
    \begin{aligned}
        \KL{\underline{p}_{(K,2),(\eta-K\Delta|0,b)}(\cdot|\vx_0,\vb)}{p_{(K,2),(\eta|0,b)}(\cdot|\vx_0,\vb)}.
    \end{aligned}
\end{equation*}
It should be noted 
\begin{equation*}
    \begin{aligned}
        &p_{(K,2),(\eta|0,b)}(\cdot|\vx_0,\vb) \propto \exp\left(-f_{\vb}(\vx)-\frac{\left\|\vx-\vx_0\right\|^2}{2\eta}\right)\\
        &\ \Rightarrow\ -\grad^2_{\vx}\ln p_{(K,2),(\eta|0,b)}(\vx|\vx_0,\vb)=\grad^2 f_{\vb}(\vx) + \frac{1}{\eta}\cdot \mI.
    \end{aligned}
\end{equation*}
When $\eta< L^{-1}$, suppose $p_{(K,2),(\eta|0,b)}(\cdot|\vx_0,\vb)$ is $\mu$ strongly log-concave.
It means $p_{(K,2),(\eta|0,b)}(\cdot|\vx_0,\vb)$ satisfies $\mu$ log-Sobolev inequality.
According to Lemma F.4 in RRDS, we have
\begin{equation*}
    \small
    \begin{aligned}
        &\KL{\underline{p}_{(K,2),(\eta-K\Delta|0,b)}(\cdot|\vx_0,\vb)}{p_{(K,2),(\eta|0,b)}(\cdot|\vx_0,\vb)}\\
        &\le \frac{1}{2\mu}\E_{\rvx\sim \underline{p}_{(K,2),(\eta-K\Delta|0,b)}(\cdot|\vx_0,\vb)}\left[\left\|\grad\log \frac{\underline{p}_{(K,2),(\eta-K\Delta|0,b)}(\rvx|\vx_0,\vb)}{p_{(K,2),(\eta|0,b)}(\rvx|\vx_0,\vb)}\right\|^2\right]\\
        &= \frac{1}{2\mu}\E_{\rvx\sim \underline{p}_{(K,2),(\eta-K\Delta|0,b)}(\cdot|\vx_0,\vb)}\left[\left\|\grad \log \frac{\left(g_{*,\vb}\ast \varphi_{K\Delta}\right)(\rvx)}{g_{*,\vb}(\rvx)} + \left(\frac{\rvx-\vx_0}{\eta} - \frac{\rvx-\vx_0}{\eta-K\Delta}\right)\right\|^2\right]\\
        &\le \frac{1}{\mu}\E_{\rvx\sim \underline{p}_{(K,2),(\eta-K\Delta|0,b)}(\cdot|\vx_0,\vb)} \left[\left\|\grad \log \frac{\left(g_{*,\vb}\ast \varphi_{K\Delta}\right)(\rvx)}{g_{*,\vb}(\rvx)}\right\|^2\right] \\
        &\quad + \frac{1}{\mu}\cdot \frac{K^2\Delta^2}{\eta^2 (\eta-K\Delta)^2}\cdot \left(\E_{\rvx\sim \underline{p}_{(K,2),(\eta-K\Delta|0,b)}(\cdot|\vx_0,\vb)} \left[\left\|\rvx-\vx_0\right\|^2\right]\right).
    \end{aligned}
\end{equation*}
It can be easily noted that, for any $\vx\in\R^d$, we have
\begin{equation*}
    \begin{aligned}
        \left\|\grad \log \frac{\left(g_{*,\vb}\ast \varphi_{K\Delta}\right)(\vx)}{g_{*,\vb}(\vx)}\right\|^2 = &\left\|\grad \log \frac{g_{*,\vb}(\vx)}{\left(g_{*,\vb}\ast \varphi_{K\Delta}\right)(\vx)}\right\|^2\\
        \le & \left(6L_{\vb}\sqrt{K\Delta}d^{1/2}+2L_{\vb}K\Delta\left\|\grad f_{\vb}(\vx)\right\|\right)^2\\
        \le & \left(6L_{\vb}\sqrt{K\Delta}d^{1/2} + 2L^2_{\vb}K\Delta\left\|\vx-\vzero\right\|+2L_{\vb}K\Delta\left\|\grad f_{\vb}(\vzero)\right\|\right)^2\\
        \le & 108L_{\vb}^2K\Delta d + 12L_{\vb}^4K^2\Delta^2 \left\|\vx\right\|^2 + 12L_{\vb}^2 K^2\Delta^2 \left\|\grad f_{\vb}(\vzero)\right\|^2
    \end{aligned}
\end{equation*}
Therefore, we have
\begin{equation*}
    \small
    \begin{aligned}
        &\KL{\underline{p}_{(K,2),(\eta-K\Delta|0,b)}(\cdot|\vx_0,\vb)}{p_{(K,2),(\eta|0,b)}(\cdot|\vx_0,\vb)}\\
        &\le \frac{1}{\mu}\E_{\rvx\sim \underline{p}_{(K,2),(\eta-K\Delta|0,b)}(\cdot|\vx_0,\vb)} \left[\left\|\grad \log \frac{\left(g_{*,\vb}\ast \varphi_{K\Delta}\right)(\rvx)}{g_{*,\vb}(\rvx)}\right\|^2\right] \\
        &\quad + \frac{1}{\mu}\cdot \frac{K^2\Delta^2}{\eta^2 (\eta-K\Delta)^2}\cdot \left(\E_{\rvx\sim \underline{p}_{(K,2),(\eta-K\Delta|0,b)}(\cdot|\vx_0,\vb)} \left[\left\|\rvx-\vx_0\right\|^2\right]\right)\\
        &\le \frac{12L_{\vb}^2 K\Delta}{\mu}\cdot \left(9d+K\Delta \left\|\grad f_{\vb}(\vzero)\right\|^2\right)+ \frac{12L_{\vb}^4 K^2\Delta^2}{\mu}\E_{\rvx\sim \underline{p}_{(K,2),(\eta-K\Delta|0,b)}(\cdot|\vx_0,\vb)}\left\|\rvx\right\|^2\\
        &\quad +\frac{1}{\mu}\cdot \frac{K^2\Delta^2}{\eta^2 (\eta-K\Delta)^2}\cdot\left(\left\|\vx_0\right\|^2+\E_{\rvx\sim \underline{p}_{(K,2),(\eta-K\Delta|0,b)}(\cdot|\vx_0,\vb)}\left\|\rvx\right\|^2\right).
    \end{aligned}
\end{equation*}
Therefore, the key point is to upper bound the second moment of $ \underline{p}_{(K,2),\eta}$ and $\underline{p}_{(K,2),0}$.
With the induction method, we are required to prove $ \underline{p}_{(K,2),\eta}$ has a bounded second moment when $\underline{p}_{(K,2),0}$ has a bounded second moment.

\section{Control the gap between the proximal oracle and an approximated RGO.}We may follow a similar idea with that shown in~\cite{liang2022proximal}.


%----------------Dec. 01--------------

We divide the second stage into several sub-stages, which correspond to the transitions among $(\bkw{\tilde{\rvx}}_0, \bkw{\tilde{\rvx}}_\tau, \ldots, \bkw{\tilde{\rvx}}_{S\tau})$ where $S\in \mathbb{N}_+$ and $S\tau = \eta$.
Hence, we introduce a variant stochastic proximal sampler.
\begin{algorithm}[!htbp]
    \caption{Stochastic Proximal Sampler}
    \label{alg:sps_var}
    \begin{algorithmic}[1]
            \State {\bfseries Input:} The negative log density $f$ of the target distribution, the initial particle $\vx_0$ drawn from $p_0$;
            \For{$k=1$ to $K$}
                \State Draw the sample $\vx_{k+1/2}$ from $\mathcal{N}(\vx_k, \eta\mI)$;
                \State Initial the particle of the inner loop as $\bkw{\vx}_0\gets \vx_{k+1/2}$;
                \For {$s=1$ to $S$}
                    \State Draw the mini-batch $\vb_{s}$ from $\{1,2,\ldots, n\}$;
                    \State Draw the sample $\bkw{\vx}_{s\tau}$ from  $\bkw{p}_{s\tau|(s-1)\tau,b}(\cdot|\vx_{(s-1)\tau},\vb_s)$;
                \EndFor
                \State Set $\vx_{k+1}\gets \bkw{\vx}_{S\tau}$;
            \EndFor
            \State {\bfseries Return:} $\vx_{K+1}$.          
    \end{algorithmic}
\end{algorithm}

In Alg~\ref{alg:sps_var}, we should note the implementation of Line 7.
Specifically, with Eq~\ref{eq:condi_TransKer_general}, we have $\bkw{\tilde{p}}_{t|t_0}(\vx|\vx_0) = \left(\bkw{\tilde{p}}_{\eta-t_0|0}(\cdot|\vx_0) \ast \varphi_{\eta - t}\right)(\vx)$, which means a particle $\bkw{\tilde{\rvx}}_{s\tau}$ sampling from $\bkw{\tilde{p}}_{s\tau|(s-1)\tau}(\cdot|\vx_{(s-1)\tau})$ can be presented as a sum of two random variables $\bkw{\tilde{\rvz}}_{s\tau}$ and $\xi_{s\tau}$ satisfying
\begin{equation*}
    \begin{aligned}
        &\bkw{\tilde{\rvz}}_{s\tau}\sim \bkw{\tilde{p}}_{\eta - (s-1)\tau|0}(\cdot|\vx_{(s-1)\tau}) = C(\eta-(s-1)\tau,\vx_{(s-1)\tau})^{-1}\cdot \exp\left(-f(\cdot) - \frac{\left\|\cdot - \vx_{(s-1)\tau}\right\|^2}{2(\eta-(s-1)\tau)}\right)\\
        &\xi_{st} \sim \mathcal{N}(\vzero, (\eta-s\tau)\cdot \mI).  
    \end{aligned}
\end{equation*}
Extend it to the randomized version, requiring a particle $\bkw{\rvx}_{s\tau}$ from $\bkw{p}_{s\tau|(s-1)\tau,b}(\cdot|\vx_{(s-1)\tau},\vb_s)$, we have the presentation $\bkw{\rvx}_{s\tau} = \bkw{\rvz}_{s\tau} + \xi_{s\tau}$ which satisfies
\begin{equation*}
    \begin{aligned}
        &\bkw{\rvz}_{s\tau}\sim \bkw{p}_{\eta - (s-1)\tau|0,b}(\cdot|\vx_{(s-1)\tau}, \vb_s) = C(\vb_s,\eta-(s-1)\tau,\vx_{(s-1)\tau})^{-1}\cdot \exp\left(-f_{\vb_s}(\cdot) - \frac{\left\|\cdot - \vx_{(s-1)\tau}\right\|^2}{2(\eta-(s-1)\tau)}\right)\\
        &\xi_{st} \sim \mathcal{N}(\vzero, (\eta-s\tau)\cdot \mI).  
    \end{aligned}
\end{equation*}
In this condition, we only consider the contraction of the last iteration and have
\begin{equation*}
    \begin{aligned}
        \KL{\tilde{p}_{K+1}}{p_{K+1}} &= \KL{\bkw{\tilde{p}}_{S\tau}}{\bkw{p}_{S\tau}} \le \KL{\bkw{\tilde{p}}_{S\tau, (S-1)\tau, b}}{\bkw{p}_{S\tau, (S-1)\tau, b}}\\
        &\le \KL{\bkw{\tilde{p}}_{(S-1)\tau}}{\bkw{p}_{(S-1)\tau}} + \E_{(\rvx, \rvb)\sim \bkw{\tilde{p}}_{(S-1)\tau, b}}\left[\KL{\bkw{\tilde{p}}_{S\tau|(S-1)\tau, b}(\cdot|\rvx,\rvb)}{\bkw{p}_{S\tau|(S-1)\tau, b}(\cdot|\rvx,\rvb)}\right]
    \end{aligned}
\end{equation*}

%-------------- Dec. 04 ------------------
Hence, we set $\eta = 1/2L$ and
    \begin{equation*}
        K= \log \frac{\KL{\tilde{p}_1}{p_*}}{2\epsilon^2}\big/\log \left(1+\frac{\alpha_*}{2L}\right) = \mathcal{\tilde{O}}(1).
    \end{equation*}
    In this condition, we have $\TVD{\tilde{p}_{K+1}}{p_*}\le \epsilon$.
    Besides, we set 
    \begin{equation*}
        B = \frac{\sigma^2 K}{2L\epsilon^2} = \mathcal{\tilde{O}}({\epsilon^{-2}})
    \end{equation*}
    Therefore, the total gradient complexity will be 
    \begin{equation*}
        K\times B = \frac{\sigma^2}{2L}\left(\log \left(1+\frac{\alpha_*}{2L}\right)\right)^{-2}\cdot \left(\log \frac{\KL{\tilde{p}_1}{p_*}}{2\epsilon^2}\right)^2\cdot \epsilon^{-2} = \mathcal{\tilde{O}}\left(\epsilon^{-2}\right).
    \end{equation*}



    With the following hyper-parameters settings, i.e.,
    \begin{equation*}
        \begin{aligned}
            \eta \le \frac{1}{2L},\quad K= \log \frac{\KL{\tilde{p}_1}{p_*}}{2\epsilon^2}\big/\log \left(1+\frac{\alpha_*}{2L}\right)\quad \mathrm{and}\quad  B = \frac{\sigma^2 K}{2L\epsilon^2},
        \end{aligned}
    \end{equation*}
    we have $\TVD{p_{K+1}}{p_*}\le 2\epsilon$. 
    In this condition, the total gradient complexity will be 
    \begin{equation*}
        \frac{\sigma^2}{2L}\left(\log \left(1+\frac{\alpha_*}{2L}\right)\right)^{-2}\cdot \left(\log \frac{\KL{\tilde{p}_1}{p_*}}{2\epsilon^2}\right)^2\cdot \epsilon^{-2} = \mathcal{\tilde{O}}\left(\epsilon^{-2}\right).
    \end{equation*}

% ---------------- Dec. 10 --------------------
We should note the first step dissipates the energy function.
    \begin{equation*}
        \begin{aligned}
            & \mathcal{E}(q_{s+\frac{1}{2}}) -\mathcal{E}(p_{1|\frac{1}{2},b}) = \int \left(q_{s+\frac{1}{2}}(\vz) - p_{1|\frac{1}{2},b}(\vz|\vx,\vb)\right)g_{\vb}(\vz) \der\vz\\
            &= \sum_{\vb_s\subseteq \vb} p(\vb_s)\cdot \int \left(q_{s+\frac{1}{2}|b}(\vz|\vb_s) - p_{1|\frac{1}{2},b}(\vz|\vx, \vb)\right)g_{\vb}(\vz)\der \vz = \mathbb{E}_{\rvb_s}\left[ \mathcal{E}(q_{s+\frac{1}{2}|b}(\cdot|\rvb_s)) - \mathcal{E}(p_{1|\frac{1}{2},b}(\cdot|\vx,\vb))\right]
        \end{aligned}
    \end{equation*}

    \textcolor{blue}{\hrule}

    For any $\rvb_s = \vb^\prime$ and $\gamma_{s}$ denotes the optimal coupling between $q_{s}$ and $p_{1|\frac{1}{2},b}(\cdot|\vx,\vb)$.
    Then, it has
    \begin{equation*}
        \begin{aligned}
            & \mathcal{E}(q_{s+\frac{1}{2}|b}(\cdot|\vb^\prime))  - \mathcal{E}(p_{1|\frac{1}{2},b})   = \E_{\rvz_s\sim q_s}\left[g_{\vb}(\rvz_s- \tau_s \grad g_{\vb^\prime}(\rvz_s))\right] - \E_{\rvz \sim p_{1|\frac{1}{2},b}}\left[g_{\vb}(\rvz)\right]\\
            &\quad  =\E_{(\rvz_s, \rvz)\sim \gamma_s}\left[g_{\vb}(\rvz_s- \tau_s \grad g_{\vb^\prime}(\rvz_s)) -  g_{\vb}(\rvz_s) + g_{\vb}(\rvz_s)-g_{\vb}(\rvz) \right]\\
            &\quad  \le \E_{(\rvz_s, \rvz)\sim \gamma_s}\left[ \left<\grad g_{\vb}(\rvz_s), -\tau_s \grad g_{\vb^\prime}(\rvz_s)\right> + \frac{3}{4\eta}\cdot \tau_s^2 \left\|\grad g_{\vb^\prime}(\rvz_s)\right\|^2 + \left<\grad g_{\vb}(\rvz_s),\rvz_s - \rvz\right> - \frac{1}{4\eta}\cdot \left\|\rvz_s - \rvz\right\|^2 \right]\\
            &\quad  = \E_{(\rvz_s,\rvz)\sim \gamma_s}\left[\left<\grad g_{\vb}(\rvz_s),\rvz_s - \tau_s \grad g_{\vb^\prime}(\rvz_s) - \rvz\right> + \frac{3}{4\eta}\cdot \tau_s^2 \left\|\grad g_{\vb^\prime}(\rvz_s)\right\|^2 - \frac{1}{4\eta}\cdot \left\|\rvz_s - \rvz\right\|^2\right].
        \end{aligned}
    \end{equation*}
    For the RHS of the previous inequality, we have
    \begin{equation*}
        \begin{aligned}
            \left\|\vz_s - \vz\right\|^2 & =\left\|\vz_s - \tau_s \grad g_{\vb^\prime}(\vz_s) - \vz_s\right\|^2 +  \left\|\vz_s - \tau_s \grad g_{\vb^\prime}(\vz_s)-\vz\right\|^2\\
            &\quad  - 2\left<\vz_s- \tau_s \grad g_{\vb^\prime}(\vz_s)-\vz_s,\vz_s -\tau_s \grad g_{\vb^\prime}(\vz_s)-\vz\right>\\
            & = \tau_s^2 \left\|\grad g_{\vb^\prime}(\vz_s)\right\|^2 + \left\|\vz_s - \tau_s \grad g_{\vb^\prime}(\vz_s) - \vz\right\|^2  + 2\left<\tau_s \grad g_{\vb^\prime}(\vz_s),\vz_s - \tau_s \grad g_{\vb^\prime}(\vz_s)-\vz\right>,
        \end{aligned}
    \end{equation*}
    which implies 
    \begin{equation*}
        \begin{aligned}
            \left<\grad g_{\vb}(\vz_s),\vz_s - \tau_s \grad g_{\vb^\prime}(\vz_s)-\vz\right> & = \left<\grad g_{\vb}(\vz_s)-\grad g_{\vb^\prime}(\vz_s),\vz_s - \tau_s \grad g_{\vb^\prime}(\vz_s)-\vz\right> + \left<\grad g_{\vb^\prime}(\vz_s),\vz_s - \tau_s \grad g_{\vb^\prime}(\vz_s)-\vz \right>\\
            & = \frac{1}{2\tau_s}\left[\left\|\vz_s-\vz\right\|^2 - \left\|\tau_s \grad g_{\vb^\prime}(\vz_s)\right\|^2 - \left\|\vz_s - \tau_s \grad g_{\vb^\prime}(\vz_s)-\vz\right\|^2\right]\\
            &\quad +\frac{1}{2\tau_s}\cdot (4\tau_s\eta) \cdot \left\|\grad g_{\vb}(\vz_s) - \grad g_{\vb^\prime}(\vz_s)\right\|^2 +  \frac{1}{2\tau_s}\cdot \frac{\tau_s}{4\eta} \left\|\vz_s - \tau_s \grad g_{\vb^\prime}(\vz_s)-\vz\right\|^2
        \end{aligned}
    \end{equation*}
    By plugging this inequality into the energy function, we have
    \begin{equation*}
        \begin{aligned}
            \mathcal{E}(q_{s+\frac{1}{2}})- \mathcal{E}(p_{1|\frac{1}{2},b})   & \le \frac{1}{2\tau_s} \E_{\gamma_s}\left[ \left(1- \frac{\tau_s}{2\eta}\right)\left\|\rvz_s-\rvz\right\|^2 - \left\|\rvz_s - \tau_s \grad g_{\vb_s}(\rvz_s)-\rvz\right\|^2 - \left(1-\frac{3\tau_s}{2\eta}\right)\tau_s^2 \left\|\grad g_{\vb_s}(\rvz_s)\right\|^2\right]\\
            & \le \frac{1}{2\tau_s}\left( \left(1- \frac{\tau_s}{2\eta}\right)W_2^2(q_s, p_{1|\frac{1}{2},b}) - \right)
        \end{aligned}
    \end{equation*}

    \textcolor{blue}{\hrule}

    Then, we have
    \begin{equation*}
        \begin{aligned}
            TB
        \end{aligned}
    \end{equation*}

% --------------- Dec. 11 -------------------------
We start with the following equation
    \begin{equation*}
        \begin{aligned}
            &\mathcal{E}(q_{s+\frac{1}{2}}) - \mathcal{E}(p_{1|\frac{1}{2},b}) = \int g(\vz) q_{s+\frac{1}{2}}(\vz)\der \vz - \int g(\vz) p_{1|\frac{1}{2},b}(\vz)\der \vz\\
            & = \sum_{\vb_s \subseteq \vb}p_b(\vb_s)\cdot \left[\int g(\vz) p_{k+\frac{1}{2}}(\vz|\vb_s)\der \vz - \int g(\vz)p_{1|\frac{1}{2},b}(\vz)\der \vz\right]\\
            & = \sum_{\vb_s \subseteq \vb} p_b(\vb_s) \cdot \int_{\gamma \in \Gamma(q_s,p_{1|\frac{1}{2},b})} \gamma(\vz_s, \vz)\cdot \left(g(\vz_s - \tau_s \grad g_{\vb_s}(\vz_s) ) - g(\vz)\right) \der (\vz_s,\vz)\\
            & = \int_{\gamma \in \Gamma(q_s,p_{1|\frac{1}{2},b})} \E_{\rvb_s}\left[g(\vz_s - \tau_s \grad g_{\rvb_s}(\vz_s)) - g(\vz)\right] \der (\vz_s, \vz)
        \end{aligned}
    \end{equation*} 
    where $\Gamma(q_s,p_{1|\frac{1}{2},b})$ denotes the coupling set between the densities $q_s$ and $p_{1|\frac{1}{2},b}$.
    Then, we start to consider each term in the integration which satisfies
    \begin{equation*}
        \begin{aligned}
            & \E_{\rvb_s}\left[g(\vz_s - \tau_s \grad g_{\rvb_s}(\vz_s))- g(\vz)\right] = \E_{\rvb_s}\left[g(\vz_s - \tau_s \grad g_{\rvb_s}(\vz_s))- g(\vz_s) + g(\vz_s)- g(\vz)\right] \\
            & \le \E_{\rvb_s}\left[-\tau_s\cdot \left<\grad g(\vz_s), \grad g_{\rvb_s}(\vz_s)\right>\right] + \E_{\rvb_s}\left[\frac{3}{4\eta}\left\|\tau_s \grad g_{\rvb_s}(\vz_s)\right\|^2\right] + \left<\grad g(\vz_s),\vz_s - \vz\right> - \frac{1}{4\eta}\left\|\vz_s - \vz\right\|^2\\
            & \le -\tau_s \left\|\grad g(\vz_s)\right\|^2 + \frac{3\tau_s^2}{2\eta}\left\|\grad g(\vz_s)\right\|^2 + \left<\grad g(\vz_s),\vz_s - \vz\right> - \frac{1}{4\eta}\left\|\vz_s - \vz\right\|^2 + \frac{3\tau_s^2}{2\eta}\E_{\rvb_s}\left[\left\|\grad g_{\rvb_s}(\vz_s) - \grad g(\vz_s)\right\|^2\right]\\
            & = -\tau_s \left\|\grad g(\vz_s)\right\|^2 + \frac{3\tau_s^2}{2\eta}\left\|\grad g(\vz_s)\right\|^2 + \left<\grad g(\vz_s),\vz_s - \vz\right> - \frac{1}{4\eta}\left\|\vz_s - \vz\right\|^2 + \frac{3\tau_s^2 \sigma^2}{2\eta |\rvb_s|},
        \end{aligned}
    \end{equation*}
    where the second inequality follows from the smoothness and strong convexity of $g(\vz)$.
    Multiplying both sides by $2\tau_s$, we have
    \begin{equation*}
        \begin{aligned}
            & 2\tau_s \cdot \E_{\rvb_s}\left[g(\vz_s - \tau_s \grad g_{\rvb_s}(\vz_s))- g(\vz)\right] \\
            & \le -\tau_s^2 \left\|\grad g(\vz_s)\right\|^2 + \frac{3\tau_s^3}{\eta}\left\|\grad g(\vz_s)\right\|^2 - \tau_s^2 \left\|\grad g(\vz_s)\right\|^2 + \left<2\tau_s\cdot \grad g(\vz_s), \vz_s - \vz\right> - \left\|\vz_s - \vz\right\|^2\\
            & \quad +\left(1- \frac{\tau_s}{2\eta}\right) \cdot \left\|\vz_s - \vz\right\|^2 + \frac{3\tau_s^3\sigma^2}{\eta|\rvb_s|}\\
            & = \left(1- \frac{\tau_s}{2\eta}\right) \cdot \left\|\vz_s - \vz\right\|^2 - \left\|\right\|^2
        \end{aligned}
    \end{equation*}

%--------------------------
\begin{lemma}[Theorem D.1 in~\cite{altschuler2023faster}]
    \label{lem:thmD1_altschuler2023faster}
    Suppose that $q_*\propto \exp(-g)$ where $g$ is $\mu$-strongly-convex and $L$-smooth. 
    Let $\vx_*$ denote the minimizer of $g$. 
    For any sampling error $\epsilon>0$ and any initialization distribution $\delta_{\vx_0} \in \mathcal{P}(\R^d)$, there is an algorithm that uses
    \begin{equation*}
        N = \tilde{O}\left(\kappa^{3/2}d^{1/2}\log(\|\vx_0-\vx_*\|)+\kappa d^{1/2}\log^3(1/\epsilon)\right)
    \end{equation*}
    first-order queries for $g$ to output a random particle in $\R^d$ with law $q_o$ satisfying $\sqrt{\chi^2(q_o\|q_*)}\le \epsilon$.
\end{lemma}

\begin{lemma}
    Using the notations presented in Alg~\ref{alg:ULD_inner}, asume~\ref{con_ass:lips_loss}-\ref{con_ass:var_bound}. 
    Alg~\ref{alg:ULD_inner} uses
    \begin{equation*}
        \tilde{O}\left(6d^{1/2}\log(3\|\vx_0\|+2\eta \|\grad f_{\vb}(\vzero)\|)+3 d^{1/2}\log^3(1/\epsilon)\right)
    \end{equation*}
    first-order queries for $g$ to output a random particle in $\R^d$ with law $q_S$ satisfying $\sqrt{\chi^2(q_S\|q_*)}\le \epsilon$.
\end{lemma}
\begin{proof}
    This proof only considers the $k$-th inner sampling subproblem, i.e., Line 5 of Alg~\ref{alg:sps}.
    The target distribution of the inner loop, i.e., $p_{k+1|k+1/2, b}(\cdot|\vx_0,\vb)$ will be abbreviated as
    \begin{equation*}
        q_{*}(\vz)\coloneqq C_q^{-1}\cdot \exp(-g(\vz)) = C_q^{-1}\cdot  \exp\left(-f_{\vb}(\vz) - \frac{\left\|\vz - \vx_0\right\|^2}{2\eta}\right).
    \end{equation*}
    In this lemma, we only consider a more explicit upper bound of gradient complexity when the $\chi^2$ error between the underlying distribution of output particles, i.e., $q_S$ and the target distribution, i.e., $q_*$ satisfying $\sqrt{\chi^2(q_S\|q_*)}\le \epsilon$.
    Specifically, if we choose $\eta\le 1/(2L)$, we have
    \begin{equation*}
        (2\eta)^{-1}\cdot \mI \preceq \grad^2 g(\vz) = \grad^2 q_*(\vz) \preceq (3/2\eta)\cdot \mI\quad \Leftrightarrow\quad \kappa \le 3
    \end{equation*}
    due to Lemma~\ref{lem:sc_sm_inner_targets}.
    Besides, the minimizer of $g$ satisfies
    \begin{equation*}
        \begin{aligned}
            \grad g(\vz_*) = \grad f_{\vb}(\vz_*)+\eta^{-1}\cdot \left(\vz_* - \vx_0\right) = \vzero \quad \Leftrightarrow \quad \vx_0 = \eta \grad f_{\vb}(\vz_*) + \vz_*,
        \end{aligned}
    \end{equation*}
    which implies
    \begin{equation*}
        \begin{aligned}
            \|\vx_0\| = \left\|\eta \grad f_{\vb}(\vz_*)+\vz_*\right\|\ge \|\vz_*\| - \eta\|\grad f_{\vb}(\vz_*)\|\quad \Leftrightarrow \quad \|\vx_0\|+\eta \|\grad f_{\vb}(\vz_*)\|\ge \|\vz_*\|.
        \end{aligned}
    \end{equation*}
    In this condition, it has
    \begin{equation*}
        \begin{aligned}
            \|\vz_*\|\le \|\vx_0\| + \eta\|\grad f_{\vb}(\vz_*) - \grad f_{\vb}(\vzero)+\grad f_{\vb}(\vzero)\|\le \|\vx_0\|+L\eta\|\vz_*\|+\eta \|\grad f_{\vb}(\vzero)\|
        \end{aligned}
    \end{equation*}
    where the second inequality follows from~\ref{con_ass:lips_loss}.
    Since, we require $L\eta\le 1/2$, then the previous inequality is equivalent to 
    \begin{equation*}
        \|\vz_*\|\le 2\|\vx_0\| + 2\eta\|\grad f_{\vb}(\vzero)\|.
    \end{equation*}
    Combining Lemma~\ref{lem:thmD1_altschuler2023faster} and Alg~\ref{alg:ULD_inner}, to require the $\chi^2$ distance between the underlying distribution of output particles $q_S$ and the inner target distribution $q_*$ to satisfy  
    \begin{equation*}
        \begin{aligned}
            \tilde{O}\left(\kappa^{3/2}d^{1/2}\log(\|\vx_0-\vx_*\|)+\kappa d^{1/2}\log^3(1/\epsilon)\right) \le \tilde{O}\left(6d^{1/2}\log(3\|\vx_0\|+2\eta \|\grad f_{\vb}(\vzero)\|)+3 d^{1/2}\log^3(1/\epsilon)\right),
        \end{aligned}
    \end{equation*}
    hence, the proof is completed.
\end{proof}

%------------------Dec. 24 -----------------------------
{\color{blue}
    \begin{theorem}
    Using the notations presented in Section~\ref{sec:not_ass_0x}, with the following hyper-parameters settings, i.e.,
    \begin{equation*}
        \begin{aligned}
            \eta \le \frac{1}{2L},\quad K= \log \frac{\KL{\tilde{p}_1}{p_*}}{2\epsilon^2}\big/\log \left(1+\frac{\alpha_*}{2L}\right),\quad \delta=\frac{\epsilon^2}{K}\quad \mathrm{and}\quad  B = \frac{\sigma^2 K}{2L\epsilon^2},
        \end{aligned}
    \end{equation*}
    we have $\TVD{p_{K+1}}{p_*}\le 3\epsilon$. 
    In this condition, the total gradient complexity will be 
    \begin{equation*}
        \frac{\sigma^2}{2L}\left(\log \left(1+\frac{\alpha_*}{2L}\right)\right)^{-2}\cdot \left(\log \frac{\KL{\tilde{p}_1}{p_*}}{2\epsilon^2}\right)^2\cdot \epsilon^{-2}\cdot \mathrm{comp}(\text{Line 5})).
    \end{equation*}
    where the last term denotes the gradient complexity for Line 5 and requires the underlying distribution $\hat{p}_{k}$ of $\hat{\rvx}_k$ to satisfy
    \begin{equation*}
        \KL{\hat{p}_{k+1|k+\frac{1}{2},b}(\cdot|\vx,\vb)}{\tilde{p}_{k+1|k+\frac{1}{2},b}(\cdot|\vx,\vb)} \le \delta = \frac{\epsilon^2}{K}
    \end{equation*}
    for any $\vx\in \R^d$ and $\vb\subseteq\{1,2,\ldots, n\}$.
\end{theorem}
\begin{proof}
    We consider to upper bound the total variation distance between $\hat{p}_{K+1}$ and $p_*$ which satisfies
    \begin{equation}
        \label{ineq:init_ineq_prac}
        \TVD{\hat{p}_{K+1}}{p_*} \le \TVD{\hat{p}_{K+1}}{p_{K+1}} + \TVD{p_{K+1}}{\tilde{p}_{K+1}}+\TVD{\tilde{p}_{K+1}}{p_*}.
    \end{equation}
    According to Lemma~\ref{lem:traj_error_cmp_norgo}, we have
    \begin{equation*}
        \TVD{\hat{p}_{K+1}}{p_{K+1}}\le \sqrt{K\delta}.
    \end{equation*}
    For the second term, by requiring $\eta\le 1/(2L)$, we have
    \begin{equation*}
        \TVD{p_{K+1}}{\tilde{p}_{K+1}}\le \sigma\sqrt{K \eta B^{-1}}.
    \end{equation*}
    Besides, for the left term in Eq~\ref{ineq:init_ineq}, we have
    \begin{equation*}
        \begin{aligned}
            \TVD{\tilde{p}_{K+1}}{p_*} \le \sqrt{\frac{1}{2}\KL{\tilde{p}_{K+1}}{p_*}}\le \sqrt{\frac{1}{2}\KL{\tilde{p}_1}{p_*}\cdot (1+\alpha_*\eta)^{-2K}}
        \end{aligned}
    \end{equation*}
    the first inequality follows from Pinsker's inequality, and the second follows from Lemma~\ref{lem:thm3_chen2022improved}.

    Hence, we set $\eta = 1/2L$ and
    \begin{equation*}
        K= \log \frac{\KL{\tilde{p}_1}{p_*}}{2\epsilon^2}\big/\log \left(1+\frac{\alpha_*}{2L}\right) = \mathcal{\tilde{O}}(1).
    \end{equation*}
    In this condition, we have $\TVD{\tilde{p}_{K+1}}{p_*}\le \epsilon$.
    Besides, we set 
    \begin{equation*}
        B = \frac{\sigma^2 K}{2L\epsilon^2} = \mathcal{\tilde{O}}({\epsilon^{-2}}),
    \end{equation*}
    which implies $\TVD{p_{K+1}}{\tilde{p}_{K+1}}\le \epsilon$.
    Additionally, we suppose $\delta = \epsilon^2/K$ and $\TVD{\hat{p}_{K+1}}{p_{K+1}}\le\epsilon$.
    Hence, the proof is completed.
    In this condition, the total gradient complexity will be
    \begin{equation*}
        K\times B \times \mathrm{comp}(\text{Line 5})) = \frac{\sigma^2}{2L}\left(\log \left(1+\frac{\alpha_*}{2L}\right)\right)^{-2}\cdot \left(\log \frac{\KL{\tilde{p}_1}{p_*}}{2\epsilon^2}\right)^2\cdot \epsilon^{-2} \cdot \mathrm{comp}(\text{Line 5}).
    \end{equation*}
\end{proof}

}


%-------------------Jan 29th ----------------

Without initialization with $\vx_*$, due to the error propagation, the gradient oracles required to achieve the convergence for Langevin-based MCMCs are dependent on the norm of both $\vx_*$ and $\vy$.
The norm of $\vx_*$ can hardly be determined, and the norm of $\vy$ should be controlled by various concentration inequalities, making their analysis complicated, and only a high probability convergence can be achieved.

In this paper, we approximate $p_*^\prime(\vx|\vy)$ with a randomized version and draw samples from it also with Langevin-based MCMCs.
We demonstrate that, with careful error propagation control, the initialization of Langevin-based MCMCs and the stochastic gradient oracles for achieving convergence will only depend on the input $\vy$.
Although the gradient complexity will be undetermined since the randomness of the input $\vy$, from an expectation perspective, it can be well upper-bounded by the second moment of particles in the entire sampling process.
Specifically, we provide two detailed implementations, benefits from the unbiased Markov chain of proximal samplers, the expected gradient complexity of these two implementations will be faster than state-of-the-art results~\cite{das2023utilising} with an $\tilde{O}(d^{1/3})$ factor at least.
